# Supplementary material for: Sherlock in OSS: A Novel Approach of Content-Based Searching in Object Storage System
Source: arXiv:2303.02105 source file (2023-05-06)
Supplement: Supplementary file 1 [file appendices.tex]

\section{Documents for Keyword Extraction}

\subsection{Document A}

This document has been collected from the SemEval2017 Dataset \cite{Augenstein2017-lq}.
The document is as followed: 

\textit{``Deep learning (also known as deep structured learning) is part of a broader family of machine learning methods based on artificial neural networks with representation learning. Learning can be supervised, semi-supervised or unsupervised.  Deep learning architectures such as deep neural networks, deep belief networks, recurrent neural networks and convolutional neural networks have been applied to fields including computer vision, machine vision, speech recognition, natural language processing, audio recognition, social network filtering, machine translation, bioinformatics, drug design, medical image analysis, material inspection and board game programs, where they have produced results comparable to and in some cases surpassing human expert  performance.  Artificial neural networks (ANNs) were inspired by information processing and distributed communication nodes in biological systems. ANNs have various differences from biological brains. Specifically, neural networks tend to be static and sym bolic, while the biological brain of most living organisms is dynamic (plastic) and analog.  The adjective "deep" in deep learning comes from the use of multiple layers in the network. Early work showed that a linear perceptron cannot be a universal classif ier, and then that a network with a nonpolynomial activation function with one hidden layer of unbounded width can on the other hand so be. Deep learning is a modern variation which is concerned with an unbounded number of layers of bounded size, which per mits practical application and optimized implementation, while retaining theoretical universality under mild conditions. In deep learning the layers are also permitted to be heterogeneous and to deviate widely from biologically informed connectionist model s, for the sake of efficiency, trainability and understandability, whence the "structured" part.''}

\noindent

\vspace{-0.4cm}

\subsection{Document B}

This document has been collected from Aarts et al. \cite{Aarts_2013}
The document is as followed: 

\textit{``Complex Langevin (CL) dynamics  {[}1,2{]} provides an approach to circumvent the sign problem in numerical simulations of lattice field theories with a complex Boltzmann weight, since it does not rely on importance sampling. In recent years a number of stimulating results has been obtained in the context of nonzero chemical potential, in both lower and four-dimensional field theories with a severe sign problem in the thermodynamic limit  {[}3–8{]} (for two recent reviews, see e.g. Refs.  {[}9,10{]}). However, as has been known since shortly after its inception, correct results are not guaranteed  {[}11–16{]}. This calls for an improved understanding, relying on the combination of analytical and numerical insight. In the recent past, the important role played by the properties of the real and positive probability distribution in the complexified configuration space, which is effectively sampled during the Langevin process, has been clarified  {[}17,18{]}. An important conclusion was that this distribution should be sufficiently localised in order for CL to yield valid results. Importantly, this insight has recently also led to promising results in nonabelian gauge theories, with the implementation of SL(N,C) gauge cooling  {[}8,10{]}.''}
